# Supplementary material for: Unbiased and Efficient Self-Supervised Incremental Contrastive Learning
Source: arXiv:2301.12104 source file (2023-01-28)
Supplement: Supplementary file 1 [file 7_Appendix.tex]

\appendix
\setcounter{theorem}{0} 
\setcounter{lemma}{0}  
\setcounter{secnumdepth}{2}
\section{Proofs}

\subsection{Proof of Equivalence}\label{app:proof_equivalence}
We first provide the proof of Theorem~\ref{th:equivalence}.

\begin{lemma}\label{lm:expection_sum}
Given $m$ sets of discrete independent random variables that are uniformly distributed, i.e. $\bigcup_{i=1}^{m} \{x_{i,j} | x_{i,j} \sim U_i(0, N_i), j=1,2,...,N_i\}$, we have
\begin{equation}
    \mathbb{E}_{x \sim U} (x) = \sum_{i=1}^m \beta_i \mathbb{E}_{x_i \sim U_i} (x_i), 
\end{equation}
where $\beta_i = N_i / \sum_{j=1}^m N_j$ and $U \coloneqq U(0, \sum_{j=1}^m N_j)$ is a uniform distribution for all variables.
\end{lemma}
\begin{proof}
The expectation of all random variables is
\begin{align}
    \mathbb{E}_{x \sim U} (x) 
    &= \sum_{i=1}^m \sum_{j=1}^{N_i} \frac{1}{\sum_{k=1}^m N_k} x_{i,j} \\
    &= \sum_{i=1}^m \sum_{j=1}^{N_i} \frac{N_i}{\sum_{k=1}^m N_k} \frac{1}{N_i} x_{i,j} \\
    &= \sum_{i=1}^m \beta_i \sum_{j=1}^{N_i} \frac{1}{N_i}  x_{i,j} \\
    &= \sum_{i=1}^m \beta_i \mathbb{E}_{x_i \sim U_i} (x_i) .
\end{align}
\end{proof}

\begin{theorem}
For old data $x_i  \in  X$, the NCE-II with the new data $\Delta X$ plus the InfoNCE only with $X$ is equivalent to the one with all data $X'$, i.e., $\mathcal{L}_i^{I,X'} = \mathcal{L}_i^{I,X} + \mathcal{L}_i^{I I}$.
\end{theorem}
\begin{proof}
For each input $x_i$, given the $\mathcal{L}^{I}_i$ in Eq.\eqref{eq:infonce} and $\mathcal{L}^{I I}_i$ in Eq.\eqref{eq:incremental_infonce}, we have
\begin{equation}
     \mathcal{L}^{I,X'}_i = - \log \frac{f_i^+}{f^+ + K \mathbb{E}_{p_n^{X'}} f_i^-},
\end{equation}
for conciseness, we use $f_i^+$ for $f(x_i,x_i^+)$ and $f_i^-$ for $f(x_i,x_i^-)$. Following Lemma~\ref{lm:expection_sum}, we have
\begin{align}
    \mathcal{L}^{I,X'}_i 
    &= - \log \frac{f_i^+}{f_i^+  +  (1 - \alpha) K \mathbb{E}_{p_n^{X}} f_i^-  +  \alpha K \mathbb{E}_{p_n^{\Delta  X}} f_i^-} \\
    &= - \log \frac{f_i^+}{f_i^+  +  K \mathbb{E}_{p_n^{X}} f_i^-  +  \alpha K (\mathbb{E}_{p_n^{\Delta  X}} f_i^-  -  \mathbb{E}_{p_n^{X}} f_i^-)} \\
    &= - (\log \frac{f_i^+}{f_i^+  +  K \mathbb{E}_{p_n^{X}} f_i^-} \nonumber \\
    & \quad\; + \log \frac{f_i^+  +  K \mathbb{E}_{p_n^{X}} f_i^-}{f_i^+  +  K \mathbb{E}_{p_n^{X}} f_i^-  +  \alpha K (\mathbb{E}_{p_n^{\Delta  X}} f_i^-  -  \mathbb{E}_{p_n^{X}} f_i^-)}) \\
    &= \mathcal{L}_i^{I,X} + \log (1 + \frac{\alpha K (\mathbb{E}_{p_n^{\Delta  X}} f_i^-  -  \mathbb{E}_{p_n^{X}} f_i^-)}{f_i^+  +  K \mathbb{E}_{p_n^{X}} f_i^-}) \\
    &= \mathcal{L}_i^{I,X} + \log (1 + \alpha \frac{f_i^+  +  K \mathbb{E}_{p_n^{\Delta  X}} f_i^-}{f_i^+  +  K \mathbb{E}_{p_n^{X}} f_i^-} - \alpha)  \\
    &= \mathcal{L}_i^{I,X} + \mathcal{L}_i^{I I}.
\end{align}
% Further, we have the total loss on the old data as
% \begin{equation}
%     \mathcal{L}^{I,X'} = \mathcal{L}^{I,X} + \mathcal{L}^{I I}
% \end{equation}
Therefore, given an encoder trained by InfoNCE on the old data, the proposed NCE-II bridges the gap caused by the change of the noise distribution and is equivalent to retraining one.
\end{proof}

\subsection{Proof of Bias Analysis}\label{app:proof_bias}
We next provide the proof of the bias analysis in Table~\ref{tab:bias}.
\begin{proof}
For inference, the bias of old data is
\begin{align}
    & \quad\; \mathcal{L}_i^{I,X} - \mathcal{L}_i^{I,X'} \nonumber \\
    &= - \log \frac{f(x_i,x_i^+)}{f(x_i,x_i^+) + K\mathbb{E}_{x_i^- \sim p_n^X} f(x_i,x_i^-)} \nonumber \\
    & \quad\; + \log \frac{f(x_i,x_i^+)}{f(x_i,x_i^+) + K\mathbb{E}_{x_i^- \sim p_n^{X'}} f(x_i,x_i^-)} \\
    &= \log f(x_i,x_i^+) + K\mathbb{E}_{x_i^- \sim p_n^X} f(x_i,x_i^-) \nonumber \\
    & \quad\; - \log f(x_i,x_i^+) + K\mathbb{E}_{x_i^- \sim p_n^{X'}} f(x_i,x_i^-) \\
    &= \log \frac{f(x_i,x_i^+) + K\mathbb{E}_{x_i^- \sim p_n^X} f(x_i,x_i^-)}{f(x_i,x_i^+) + K\mathbb{E}_{x_i^- \sim p_n^{X'}} f(x_i,x_i^-)} \\
    &= r_{i,X \to X'}.
\end{align}
And the bias of new data is self-evidence. For fine-tuning, the bias of old data is the same as inference and the bias of new data is
\begin{align}
    & \quad\; \mathcal{L}_i^{I,\Delta X} - \mathcal{L}_i^{I,X'} \nonumber \\
    &= - \log \frac{f(x_i,x_i^+)}{f(x_i,x_i^+) + K\mathbb{E}_{x_i^- \sim p_n^{\Delta X}} f(x_i,x_i^-)} \nonumber \\
    & \quad\; + \log \frac{f(x_i,x_i^+)}{f(x_i,x_i^+) + K\mathbb{E}_{x_i^- \sim p_n^{X'}} f(x_i,x_i^-)} \\
    &= \log f(x_i,x_i^+) + K\mathbb{E}_{x_i^- \sim p_n^{\Delta X}} f(x_i,x_i^-) \nonumber \\
    & \quad\; - \log f(x_i,x_i^+) + K\mathbb{E}_{x_i^- \sim p_n^{X'}} f(x_i,x_i^-) \\
    &= \log \frac{f(x_i,x_i^+) + K\mathbb{E}_{x_i^- \sim p_n^{\Delta X}} f(x_i,x_i^-)}{f(x_i,x_i^+) + K\mathbb{E}_{x_i^- \sim p_n^{X'}} f(x_i,x_i^-)} \\
    &= r_{i,\Delta X \to X'}.
\end{align}
\end{proof}

\subsection{Proof of Bound}\label{app:proof_bound}
We next give the proof of Theorem~\ref{th:bound}.

\begin{theorem}
The difference between the empirical risk of the method with the proposed NCE-II and retraining with InfoNCE in the entire training process is bounded by $\alpha \mathcal{R}^{old}$, where $\mathcal{R}^{old}=\frac{1}{N}\sum_{i=1}^N \mathcal{L}_i^{I,old}$ approaches to zero as $\mathcal{L}_i^{I,old}$ is minimized after previous training process on old data $X$ and the growth ratio $\alpha \in [\,0,1)$. Then we have $\alpha \mathcal{R}^{old} \to 0$.
\end{theorem}
\begin{proof}
In the whole training process, the empirical risk of the proposed incremental method is
\begin{align}
    \mathcal{R} 
    &= \mathcal{R}^{old} + \mathcal{R}^{inc} \\
    &= \frac{1}{N} \sum_{x_i \in X} \mathcal{L}_i^{I,X} + \frac{1}{N  +  \Delta  N} \mathcal{L}.
\end{align}

The empirical risk of retraining is
\begin{align}
    \mathcal{R}^{retrain} 
    &= \frac{1}{N  +  \Delta  N} \sum_{x_i \in X'} \mathcal{L}_i^{I,X'} \\
    &= \frac{1}{N  +  \Delta  N} (\sum_{x_i \in X} \mathcal{L}_i^{I,X'}  +     \sum_{x_i \in \Delta X} \mathcal{L}_i^{I,X'}) \\
    &= \frac{1}{N  +  \Delta  N} (\sum_{x_i \in X} \mathcal{L}_i^{I,X}  +     \sum_{x_i \in X} \mathcal{L}_i^{I I}  +     \sum_{x_i \in \Delta X} \mathcal{L}_i^{I,X'}).
\end{align}

Thus, the difference between the proposed method and retraining is
\begin{align}
    \Delta \mathcal{R} 
    = \mathcal{R} - \mathcal{R}^{retrain}  = \alpha \mathcal{R}^{old}.
\end{align}
Therefore, the bound is $\alpha \mathcal{R}^{old}$, where $\mathcal{R}^{old}$ approaches to zero since the origin training process on the old data $X$ converges and is weighted by the growth ratio $\alpha \in [\,0,1)$. That is, $\alpha \mathcal{R}^{old} \to 0$.
\end{proof}

\section{Learning Rate Learning Optimization}
For LRL, we optimize the critic network using Temporal-Difference (TD) learning on a random-sampled mini-batch of $M$ transitions $(s_t, a_t, r_t, s_{t+1})$ stored in a replay buffer:
\begin{equation}\label{eq:update_critic}
    \mathcal{L}^Q = \frac{1}{M} \sum_{i=1}^M (y_i-Q(s_i,a_i|\theta^Q))^2,
\end{equation}
where $y_i = r_i + \gamma Q'(s_{i+1}, \mu'(s_{i+1}|\theta^{\mu'})|\theta^{Q'})$ represents the TD target and $\gamma$ is the discount parameter.
The actor network are updated by applying the chain rule:
\begin{equation}\label{eq:update_actor}
    \nabla_{\theta^\mu} = \frac{1}{M} \sum_{i=1}^M \cdot \nabla_a Q(s_i,\mu(s_i|\theta^\mu)|\theta^Q) \nabla_{\theta^\mu} \mu(s_i|\theta^\mu),
\end{equation}
And the target networks are updated using
\begin{align}\label{eq:update_target}
    \theta^{Q'} \gets m \theta^Q &+ (1-m) \theta^{Q'}, \\
    \theta^{\mu'} \gets m \theta^\mu &+ (1-m) \theta^{\mu'},
\end{align}
where $m$ is the momentum term.

Finally, we use the LRL mechanism to generate the learning rates in meta-optimization according to the status of the training process.

\begin{algorithm}[t]
\caption{Incremental Contrastive Learning}\label{alg:icl}
\LinesNumbered 
\KwIn{old data $X$ and new data $\Delta X$, encoder $\phi(x;\theta)$ trained on $X$, number of negative samples $K$, growth rate $\alpha$, DDPG networks $\mathcal{D}$ for $X$ and $\mathcal{D'}$ for $\Delta X$}
\KwOut{encoder $\phi(x;\theta)$}
\While{not converge}{
    \ForEach{$x_i \in \Delta X$}{
        \tcp{meta-train}
        let $\theta'=\theta$ \;
        \ForEach{$x_j \in $ sampled $\{x_j\}_{j=1}^{\lceil ( 1 - \alpha ) / \alpha \rceil}$ from $X$}{
            get positive $x_j^+$ with augmentation \;
            sample negatives $\{x_{j,k}^-\}_{k=1}^K \sim p_n^X,  \{x_{j,k}^-\}_{k=K}^{2K} \sim p_n^{\Delta X}$\;
            get the embeddings with $\phi(x;\theta')$ \;
            calculate $\mathcal{L}_j^{I I} \gets$ Eq.\eqref{eq:incremental_infonce} \;
            extract state $s_j = \mathcal{F}(x_j, \theta')$ \;
            generate learning rate $lr_s \gets$ Eq.\eqref{eq:generate_learning_rate} \;
            calculate new parameters $\theta' \gets$ Eq.\eqref{eq:update_parameters} \;
            get the reward $r_j \gets$ Eq.\eqref{eq:reward} \;
            update $\mathcal{D} \gets$ Eq.\eqref{eq:update_critic} $\sim$ Eq.\eqref{eq:update_target} \;
        }
        \tcp{meta-test}
        get positive $x_i^+$ with augmentation \;
        sample negatives $\{x_{i,k}^-\}_{k=1}^K \sim p_n^{X'}$\;
        get the embeddings with $\phi(x;\theta')$ \;
        calculate $\mathcal{L}_i^{I,X'} \gets$ Eq.\eqref{eq:infonce} \;
        extract state $s_i = \mathcal{F}(x_i, \theta')$ \;
        generate learning rate $lr_q \gets$ Eq.\eqref{eq:generate_learning_rate} \;
        update parameters $\theta \gets$ Eq.\eqref{eq:update_parameters} \;
        get the reward $r_i \gets$ Eq.\eqref{eq:reward} \;
        update $\mathcal{D'} \gets$ Eq.\eqref{eq:update_critic} $\sim$ Eq.\eqref{eq:update_target} \;
    }
}
\end{algorithm}
